# Supplementary material for: Separable and Localized System Level Synthesis for Large-Scale Systems
Source: arXiv:1701.05880 source file (2017-01-20)
Supplement: Supplementary file 1 [file Appendix_A.tex]

%\section*{APPENDIX}
The key point to prove Theorem \ref{thm:local_feasibility} is showing that \eqref{eq:freq_col} is feasible if and only if \eqref{eq:freq_local} is feasible for each $j$. For $\ell = (j,d)$, we define the embedding linear operators $E_x(\cdot)$ on $x_\ell$ and $E_u(\cdot)$ on $u_\ell$, which simply add appropriate zero padding such that $E_x(x_\ell[k]) = (R[k])_j$ and $E_u(u_\ell[k]) = (M[k])_j$. In particular, we have that $E_x(e_\ell) = e_j$. For a $(d,T)$ localized FIR constraint $(\mathcal{S}_R, \mathcal{S}_M)$, we have the following lemma.
%The following lemma is useful to prove Theorem 1. We assume that $(\mathcal{S}_x, \mathcal{S}_u)$ is a $(d,T)$ localized FIR constraint for $(A,B)$.
\begin{lemma}
Suppose that $\Sp{x_\ell} \subseteq \mathcal{S}_{x \ell}$ and $\Sp{u_\ell} \subseteq \mathcal{S}_{u \ell}$. Then 
\begin{equation}
E_x(A_{\ell} x_\ell[k]) = A E_x(x_\ell[k])\label{eq:lem1}
\end{equation}
\begin{equation}E_x(B_{2 \ell} u_\ell[k]) = B_2 E_u(u_\ell[k]).\label{eq:lem2}
\end{equation}
\label{lemma:local_feasibility}
\end{lemma}
\begin{proof}
We only prove equality \eqref{eq:lem1}, as \eqref{eq:lem2} follows from a nearly identical argument.
The constraint $\Sp{x_\ell} \subseteq \mathcal{S}_{x \ell}$ implies that the support of $E_x(x_\ell[k])$ is contained within $Down(j,d)$. Let $x_i$ be a state such that $i \not\in Down(j,d+1)$ and $x_k$ a state such that $\dist{h}{i}{\A} \leq 1$: then $h \not\in Down(j,d)$. Let $\Delta_{A1}$ be a matrix of the same dimension as $A$, but only have one (possibly) non-zero entry $-A_{ih}$ at $(i,h)$-th location. Clearly, $\Delta_{A1} E_x(x_\ell[k]) = 0$. Therefore, setting the $(i,h)$-entry of $A$ to zero does not change the value of the RHS of \eqref{eq:lem1}. 

Similarly, let $x_s$ be a state such that  $\dist{i}{s}{\A} \leq 1$. Letting $\Delta_{A2}$ be a matrix of the same dimension as $A$, but with only one (possibly) non-zero entry $-A_{si}$ at $(s,i)$-th location, we then also have $\Delta_{A2} E_x(x_\ell[k]) = 0$ for all $k$.  Thus setting the $(s,i)$-entry of $A$ to zero does not change the value of the RHS of \eqref{eq:lem1}. 

Repeatedly applying this argument, we can explicitly set all the elements in the $i$-th row/column of $A$ to zero for all $i \not\in Down(j,d+1)$, without changing the value of the RHS of \eqref{eq:lem1}. This clearly implies that the desired equality indeed holds from the definition of $A_\ell$. 
\end{proof}

Now, we can prove Theorem \ref{thm:local_feasibility}.

\begin{proof}[Theorem \ref{thm:local_feasibility}]
Assume that $(x_\ell,u_\ell)$ is a feasible solution for \eqref{eq:freq_local}. Applying the $E_x$ operator to both sides of \eqref{eq:freq_local} and using Lemma \ref{lemma:local_feasibility}, it is straightforward to verify that $(E_x(x_\ell),E_u(u_\ell))$ satisfy \eqref{eq:freq_col}. In addition, $E_x(x_\ell) \in (\mathcal{S}_R)_j$ and $E_u(u_\ell) \in (\mathcal{S}_M)_j$, so the global feasibility test is feasible.

To show the opposite direction, assume that $(R,M)$ is a solution to the global feasibility test. It suffices to show that $(R_j,M_j)$ satisfy the same sparsity constraints as $(E_x(x_\ell),E_u(u_\ell))$. This directly follows from the column-wise interpretation of a $(d,T)$ localized FIR constraint $(\mathcal{S}_R, \mathcal{S}_M)$ for $(A,B_2)$.
\end{proof}
